# Supplementary material for: On biological flow networks: Antagonism between hydrodynamic and metabolic stimuli as driver of topological transitions
Source: arXiv:2111.04326 source file (2021-11-15)
Supplement: Supplementary file 1 [file S1-modelAbsorption.tex]

% % % % % % % % % % % % % % % % % % % % % % % %

\documentclass[10pt,letterpaper]{article}
\usepackage[left=0.9in, right=0.9in,]{geometry}
% amsmath and amssymb packages, useful for mathematical formulas and symbols
\usepackage{amsmath,amssymb}

% Use adjustwidth environment to exceed column width (see example table in text)
\usepackage{changepage}

% Use Unicode characters when possible
\usepackage[utf8x]{inputenc}

% textcomp package and marvosym package for additional characters
\usepackage{textcomp,marvosym}

% cite package, to clean up citations in the main text. Do not remove.
\usepackage{cite}

% Use nameref to cite supporting information files (see Supporting Information section for more info)
\usepackage{nameref,hyperref}

% line numbers
\usepackage[right]{lineno}

% ligatures disabled
\usepackage{microtype}
\DisableLigatures[f]{encoding = *, family = * }

% color can be used to apply background shading to table cells only
\usepackage[table]{xcolor}

% array package and thick rules for tables
\usepackage{array}

% create "+" rule type for thick vertical lines
\newcolumntype{+}{!{\vrule width 2pt}}

% create \thickcline for thick horizontal lines of variable length
\newlength\savedwidth

% \thickhline command for thick horizontal lines that span the table

% Remove comment for double spacing
\usepackage{setspace} 
\doublespacing

% Text layout
%\raggedright
%\setlength{\parindent}{0.5cm}
%\textwidth 5.25in 
%\textheight 8.75in

% Bold the 'Figure #' in the caption and separate it from the title/caption with a period
% Captions will be left justified
\usepackage[aboveskip=1pt,labelfont=bf,labelsep=period,justification=raggedright,singlelinecheck=off]{caption}

% Use the PLoS provided BiBTeX style
\bibliographystyle{plos2015}

% Remove brackets from numbering in List of References
\makeatletter
\renewcommand{\@biblabel}[1]{\quad#1.}
\makeatother

% Header and Footer with logo
\usepackage{lastpage,fancyhdr,graphicx}
\usepackage{epstopdf}
\pagestyle{fancy}
\fancyhf{}
%\setlength{\headheight}{27.023pt}
%\lhead{\includegraphics[width=2.0in]{PLOS-submission.eps}}
%\rfoot{\thepage/\pageref{LastPage}}
%\renewcommand{\headrulewidth}{0pt}
%\renewcommand{\footrule}{\hrule height 2pt \vspace{2mm}}
%\fancyheadoffset[L]{2.25in}
%\fancyfootoffset[L]{2.25in}
%\lfoot{\today}

\input{../packages}
\input{../macros}
%% END MACROS SECTION

%%remove figures for submission, because plos is weird
\usepackage{comment}
\excludecomment{versiona}
\includecomment{versionb}
\begin{document}

\begin{LARGE}
\textbf{S1 Appendix: Metabolite transport in arbitrary Kirchhoff networks}
\end{LARGE}

In this section we shall give a detailed run-down of the derivation of the equations systems and solutions in section 1. The continuity equation was reading in the non-dimensional form as
\alg{
	 \bar{c}\bra{z^*}= & X_{0} \e^{ \lambda_{+} z^* }+X_{1}\e^{ \lambda_{-} z^*}\\
	\text{with }\lambda_{\pm} &= \frac{1}{2}\bra{ Pe \pm\sqrt{Pe^2 + \beta^*  }}
}

with channels boundaries $\bar{c}\bra{z=0}=\bar{c}_0$, $\bar{c}\bra{z=L}=\bar{c}_L$ and $X_{0}=\frac{\bar{c}_L-\bar{c}_0\e^{a_{1}}}{\e^{a_0}-\e^{a_1}}$, $ X_{1}=\frac{\bar{c}_0\e^{a_{0}}-\bar{c}_L}{\e^{a_0}-\e^{a_1}}$.
In order to calculate the solute flux and the corresponding equations system for a complex network one writes (using $x_e=\sqrt{Pe_e^2 + \beta^*_e }$)
\alg{
	I_k\bra{z}= A_k \bra{ \bar{u}_k\bar{c}_k\bra{z} - D\partd{z}\bar{c}_k\bra{z} }=\frac{A_k D}{L}\bra{ Pe_k\bar{c}_k\bra{z}-\partd{z^*}\bar{c}_k\bra{z} }\\
	\Rightarrow I_k\bra{0}=I_{\alpha\bra{k}}=\frac{A_k D}{2L}\bro{ \bar{c}_{\alpha\bra{k}}\brc{Pe_k + x_k \coth\bra{\frac{x_k}{2}}} -\bar{c}_{\omega\bra{k}} \frac{x_k\e^{-\frac{Pe_k}{2}}}{\sinh\bra{\frac{x_k}{2}}}}\\
	\Rightarrow I_k\bra{L}=I_{\omega\bra{k}}=\frac{A_k D}{2L}\bro{ \bar{c}_{\omega\bra{k}}\brc{Pe_k - x_k \coth\bra{\frac{x_k}{2}}} +\bar{c}_{\alpha\bra{k}} \frac{x_k\e^{\frac{Pe_k}{2}}}{\sinh\bra{\frac{x_k}{2}}}}
}
Now we utilize the the boundary conditions for solute flux on every node as, using  $\frac{A_k D}{L}=q_k$ as an abbreviation, so that we write for in- and outflux of solute of a vertex:
\alg{
J_i &=\sum_k B_{ik}I_k=\sum_{k\in out(i)} I_{\alpha\bra{k}} - \sum_{k\in in(i)} I_{\omega\bra{k}}\\
&=  \sum_k  q_k\bra{B_{ik}Pe_k + \vert B_{ik} \vert x_k \coth\bra{\frac{x_k}{2}}}\bar{c}_i\nonumber\\ &-\sum_{k\in out(i)}q_k\frac{x_k\e^{-\frac{Pe_k}{2}}}{2 \sinh\bra{\frac{x_k}{2}}}\bar{c}_{\omega\bra{k}} - \sum_{k\in in(i)}q_k \frac{x_k\e^{\frac{Pe_k}{2}}}{2\sinh\bra{\frac{x_k}{2}}}\bar{c}_{\alpha\bra{k}}
}
We may rewrite this equation system according to \cite{1988PhRvA..37.2619K} in vectorial form,
\g{
 \vc{M}\cdot\vc{c}=\vc{J}
}
which also allows us to efficiently solve for $\vc{c}$ for any given $\vc{J}$ with
\alg{
M_{ij}&= \sum_k  \frac{q_k}{2}\brc{B_{ik}Pe_k + \vert B_{ik} \vert x_k  \coth\bra{\frac{x_k}{2}}}\delta_{ij} -\sum_{k\in out(i)}q_k \frac{x_k\e^{-\frac{Pe_k}{2}}}{2\sinh\bra{\frac{x_k}{2}}}\delta_{\omega\bra{k},j}- \sum_{k\in in(i)}q_k \frac{x_k\e^{\frac{Pe_k}{2}}}{2\sinh\bra{\frac{x_k}{2}}}\delta_{\alpha\bra{k},j}
}
As we generally utilize mixed boundary conditions with $c_n=0$ on the outflux periphery and $J_n>0$ on the influx periphery of the network we can calculate the complementary missing values and subsequently calculate the linkwise metabolite absorption as,
\alg{
\Phi &=\sum_i J_i \\ &=\sum_k \frac{q_k}{2}\bro{ \bar{c}_{\alpha\bra{k}}\brc{ x_k \coth\bra{\frac{x_k}{2}} - \frac{x_k\e^{\frac{Pe_k}{2}}}{\sinh\bra{\frac{x_k}{2}}} +Pe_k}  + \bar{c}_{\omega\bra{k}}\brc{ x_k \coth\bra{\frac{x_k}{2}} - \frac{x_k\e^{-\frac{Pe_k}{2}}}{\sinh\bra{\frac{x_k}{2}}} - Pe_k} }\\
 \Rightarrow \Phi_k &= \frac{q_k}{2}\bro{ \bar{c}_{\alpha\bra{k}}\brc{ x_k \coth\bra{\frac{x_k}{2}} - \frac{x_k\e^{\frac{Pe_k}{2}}}{\sinh\bra{\frac{x_k}{2}}} +Pe_k}  + \bar{c}_{\omega\bra{k}}\brc{ x_k \coth\bra{\frac{x_k}{2}} - \frac{x_k\e^{-\frac{Pe_k}{2}}}{\sinh\bra{\frac{x_k}{2}}} - Pe_k} }
}
In Fig. \ref{fig:apx_solute_solution_1} we display an examplary solution for a single channel with absorbing boundary. 
One finds the concentrations profile in general to become linear in the case of small Peclet numbers, corresponding to the maximal possible decline in solute flux, see \ref{fig:solutions_cI}. 
Further to get a quantitative and qualitative perspective on the metabolite uptake in this system one may consider the effective uptake, see \ref{fig:solutions_phi}. 
As depicted one finds the uptake to vary drastically with the Peclet numbers as well as the effective absorption rate. Note  that increased Peclet numbers generally correspond to a decreased uptake while entering the diffusive regime for $Pe \rightarrow 0$ displays clear saturation behavior in dependence of $\beta^*$ .
\begin{figure}[ht!]
\begin{versionb}
\subfloat{
\label{fig:solutions_cI}}
\subfloat{
 \label{fig:solutions_phi}}
\caption{Single channel solutions with absorbing boundary: \subR{fig:solutions_cI} Concentration and solute flux profiles for ${\beta^*=10^{-2}}$ \subR{fig:solutions_phi} Effective metabolite uptake }\label{fig:apx_solute_solution_1}
\end{versionb}

\begin{versiona}
\subfloat[]{
\hspace{-1cm}\includegraphics[scale=1.]{../Figures_Supplement/concentration_constant_beta}
 \label{fig:solutions_cI}}
\subfloat[]{
\includegraphics[scale=1.]{../Figures_Supplement/phi_profile_absorbing}
 \label{fig:solutions_phi}}
\caption{Single channel solutions with absorbing boundary: \subR{fig:solutions_cI} Concentration and solute flux profiles for ${\beta^*=10^{-2}}$ \subR{fig:solutions_phi} Effective metabolite uptake }\label{fig:apx_solute_solution_1}
\end{versiona}
\end{figure}

\end{document}
