# Supplementary material for: On biological flow networks: Antagonism between hydrodynamic and metabolic stimuli as driver of topological transitions
Source: arXiv:2111.04326 source file (2021-11-15)
Supplement: Supplementary file 2 [file S2-jacobianAdaptation.tex]

% % % % % % % % % % % % % % % % % % % % % % % %

\documentclass[10pt,letterpaper]{article}
\usepackage[left=0.9in, right=0.9in,]{geometry}
% amsmath and amssymb packages, useful for mathematical formulas and symbols
\usepackage{amsmath,amssymb}

% Use adjustwidth environment to exceed column width (see example table in text)
\usepackage{changepage}

% Use Unicode characters when possible
\usepackage[utf8x]{inputenc}

% textcomp package and marvosym package for additional characters
\usepackage{textcomp,marvosym}

% cite package, to clean up citations in the main text. Do not remove.
\usepackage{cite}

% Use nameref to cite supporting information files (see Supporting Information section for more info)
\usepackage{nameref,hyperref}

% line numbers
\usepackage[right]{lineno}

% ligatures disabled
\usepackage{microtype}
\DisableLigatures[f]{encoding = *, family = * }

% color can be used to apply background shading to table cells only
\usepackage[table]{xcolor}

% array package and thick rules for tables
\usepackage{array}

% create "+" rule type for thick vertical lines
\newcolumntype{+}{!{\vrule width 2pt}}

% create \thickcline for thick horizontal lines of variable length
\newlength\savedwidth

% \thickhline command for thick horizontal lines that span the table

% Remove comment for double spacing
\usepackage{setspace} 
\doublespacing

% Text layout
%\raggedright
%\setlength{\parindent}{0.5cm}
%\textwidth 5.25in 
%\textheight 8.75in

% Bold the 'Figure #' in the caption and separate it from the title/caption with a period
% Captions will be left justified
\usepackage[aboveskip=1pt,labelfont=bf,labelsep=period,justification=raggedright,singlelinecheck=off]{caption}

% Use the PLoS provided BiBTeX style
\bibliographystyle{plos2015}

% Remove brackets from numbering in List of References
\makeatletter
\renewcommand{\@biblabel}[1]{\quad#1.}
\makeatother

% Header and Footer with logo
\usepackage{lastpage,fancyhdr,graphicx}
\usepackage{epstopdf}
\pagestyle{fancy}
\fancyhf{}
%\setlength{\headheight}{27.023pt}
%\lhead{\includegraphics[width=2.0in]{PLOS-submission.eps}}
%\rfoot{\thepage/\pageref{LastPage}}
%\renewcommand{\headrulewidth}{0pt}
%\renewcommand{\footrule}{\hrule height 2pt \vspace{2mm}}
%\fancyheadoffset[L]{2.25in}
%\fancyfootoffset[L]{2.25in}
%\lfoot{\today}

%% END MACROS SECTION
\input{../packages}
\input{../macros}
%%remove figures for submission, because plos is weird
\usepackage{comment}
\excludecomment{versiona}
\includecomment{versionb}

\begin{document}

\begin{LARGE}
\textbf{S2 Appendix: Demand-supply based adaptation algorithm}
\end{LARGE}

Now we formulate a dynamical system which shall describe the adaptation of a vessel network in order to minimize the metabolic cost function $\Gamma$:
\g{
	\Gamma=S\bra{ \vc{\Phi},\vc{\Phi}_0} + \sum_e\bra{  \alpha_1 \frac{f^2_e}{K_e} +\alpha_0 K_e^{\gamma}}
}
%So we formulate the equations of motions as 
%\alg{
%	\rightarrow \partd{t} \vc{r} = -\chi \nabla{r} \Gamma =-\chi \vc{D}_S \cdot \vc{D}_{\Phi}+ \vc{D}_T\cdot \vc{D}_K
%}
Following the gradient-descent approach in order reach Lyapunov stable states we formulate the equations of motions as,
\alg{
	 \partd{t} r_i & = -\chi \partd{r_i} \Gamma \\&=-\chi \sum_j\partd{\Phi_j}S\bra{ \vc{\Phi},\vc{\Phi}_0}\partd{r_j}\Phi + \partd{r_i}\sum_e \bra{ \alpha_1 \frac{f^2_e}{K_e} +\alpha_0 K_e^{\gamma}}\label{eq:apx_eq_motion}
}
with an arbitrary $\chi >0$ to ensure $\partd{t}\Gamma \leq 0$. 
The last term in Eq. \eqref{eq:apx_eq_motion}, concerning the derivatives of the dissipation-volume costs, has been discussed in previous studies , e.g. \cite{PhysRevResearch.2.043171}. Subsequently we proceed with the metabolic uptake problem. 
First, we rewrite the uptake term $\Phi_k$ for an arbitrary link $k$ as 
\alg{
\Phi_k &= \frac{q_k}{2}\bra{ \bar{c}_{\alpha\bra{k}} G_k  + \bar{c}_{\omega\bra{k}} H_k  }
}
with sub-functions defined as,
\alg{
G_k&=\bra{ x_k \coth\bra{\frac{x_k}{2}} - \frac{x_k\e^{\frac{Pe_k}{2}}}{\sinh\bra{\frac{x_k}{2}}} +Pe_k}\\
H_k&=\bra{ x_k \coth\bra{\frac{x_k}{2}} - \frac{x_k\e^{-\frac{Pe_k}{2}}}{\sinh\bra{\frac{x_k}{2}}} - Pe_k}
}
and partial derivatives (using notation $\partd{r_j} \bra{\cdot}=\partd{j} \bra{\cdot}$) are calcuated as 
\alg{
	\partd{j}\Phi_k &=\partd{j} \frac{q_k}{2}\bra{ \bar{c}_{\alpha\bra{k}} G_k  + \bar{c}_{\omega\bra{k}} H_k  }+\frac{q_k}{2}\bra{ \partd{j}\bar{c}_{\alpha\bra{k}} G_k  + \partd{j}\bar{c}_{\omega\bra{k}} H_k  }+\frac{q_k}{2}\bra{ \bar{c}_{\alpha\bra{k}} \partd{j}G_k  + \bar{c}_{\omega\bra{k}} \partd{j}H_k  }\\
	\partd{j}q_k &=2\pi R_k\delta_{jk}\\
	\partd{j}c_i &=\partd{j}\bra{\vc{e}_i^T\cdot\vc{c}}=\vc{e}_i^T\cdot\partd{j}\bra{\vc{M}^{\dagger}\vc{J}}=-\vc{e}_i^T\cdot\bra{\vc{M}^{\dagger}\partd{j}\vc{M}\vc{M}^{\dagger}\vc{J}}=-\vc{e}_i^T\cdot\bra{\vc{M}^{\dagger}\partd{j}\vc{M}\vc{c}}}
Subsequently we can calulate the derivates of $\vc{M}$ and the sub-components as	
	\g{
	\partd{j}M_{ij}= \sum_k  \partd{j}\frac{q_k}{2}\brc{B_{ik}Pe_k + \vert B_{ik} \vert x_k  \coth\bra{\frac{x_k}{2}}}  \delta_{ij} \nonumber \\
+	\sum_k  \frac{q_k}{2}\bra{ B_{ik}  + \vert B_{ik} \vert \bro{ \frac{\coth\bra{\frac{x_k}{2}}}{x_k} - \brc{  \frac{\coth\bra{\frac{x_k}{2}}}{\cosh\bra{\frac{x_k}{2}}} }^2}}\partd{j}Pe_k\delta_{ij}\nonumber \\
 -\sum_{k\in out(i)} \bro{ \partd{j}\frac{q_k}{2} \frac{x_k\e^{-\frac{Pe_k}{2}}}{\sinh\bra{\frac{x_k}{2}}} + \frac{q_k}{2} \frac{\e^{-\frac{Pe_k}{2}}}{\sinh\bra{\frac{x_k}{2}}}\brc{ \frac{Pe_k}{x_k} -\frac{x_k}{2} -\frac{Pe_k}{2}\coth\bra{\frac{x_k}{2}}}\partd{j}Pe_k}\delta_{\omega\bra{k},j}\nonumber\\
-\sum_{k\in in(i)} \bro{ \partd{j}\frac{q_k}{2} \frac{x_k\e^{-\frac{Pe_k}{2}}}{\sinh\bra{\frac{x_k}{2}}} + \frac{q_k}{2} \frac{\e^{-\frac{Pe_k}{2}}}{\sinh\bra{\frac{x_k}{2}}}\brc{ \frac{Pe_k}{x_k} +\frac{x_k}{2} -\frac{Pe_k}{2}\coth\bra{\frac{x_k}{2}}}\partd{j}Pe_k}\delta_{\alpha\bra{k},j}\\
\partd{j}G_k=\frac{\partd{j}Pe_k}{\sinh\bra{\frac{x_k}{2}}}\bro{ \frac{Pe_k}{x_k}\brc{ \cosh\bra{\frac{x_k}{2}} - \e^{\frac{Pe_k}{2}}} + \sinh\bra{\frac{x_k}{2}} -\frac{Pe_k}{2\sinh\bra{\frac{x_k}{2}}} +\e^{\frac{Pe_k}{2}}\brc{ \frac{Pe_k}{2}\coth\bra{\frac{x_k}{2}}- \frac{x_k}{2}}}\\
\partd{j}H_k=\frac{\partd{j}Pe_k}{\sinh\bra{\frac{x_k}{2}}}\bro{ \frac{Pe_k}{x_k}\brc{ \cosh\bra{\frac{x_k}{2}} - \e^{-\frac{Pe_k}{2}}} - \sinh\bra{\frac{x_k}{2}}  -\frac{Pe_k}{2\sinh\bra{\frac{x_k}{2}}} +\e^{-\frac{Pe_k}{2}}\brc{ \frac{Pe_k}{2}\coth\bra{\frac{x_k}{2}} + \frac{x_k}{2}}}
}
Finally we calculate the derivates of the local Peclet numbers as
\g{
\partd{j}Pe_k=\frac{L_k}{D}\partd{j}\bar{u}_k \text{ with } \partd{j}\bar{u}_k=\partd{j}\bra{\frac{R^2_k\LP p_k}{8\eta L_k}}=\frac{1}{8\eta L_k}\bra{ 2\delta_{jk}R_k \LP p_k + R_k^2\partd{j}\LP p_k }
}
We compute the pressure derivatives from the Kirchhoff solutions as 
\alg{
 \partd{j}\LP p_k &=\partd{j}\brc{ \vc{e}_k ^T\vc{B}^T\bra{  \vc{B} \vc{C} \vc{B}^T }^{\dagger} \vc{s}}\\
 &=- \vc{e}_k^T \vc{B}^T\brc{\vc{B} \vc{C} \vc{B}^T }^{\dagger}\vc{B} \partd{j}\vc{C} \LP\vc{p}\\
&=- \vc{e}_k^T \vc{B}^T\brc{\vc{B} \vc{C} \vc{B}^T }^{\dagger}\vc{B}\brc{ \frac{4C_j}{R_j} \bra{\vc{e}_j\otimes\vc{e}_j}}\LP\vc{p}\\
&=- \frac{4C_j \LP p_j}{R_j} \bra{ \vc{B}^T\brc{\vc{B} \vc{C} \vc{B}^T }^{\dagger}\vc{B}}_{jk}
}
which closes the system derivatives for $\partd{t}r_i$ and allows us to evaluate the flow landscape as well as the occuring gradients accordingly. 
For numerical purposes, one is remined to carefully evaluate Peclet number dependend exponential and hyperbolical functions as overflow errors are likely to occur. 
%This kind of problem can easily be avoided, when approximated and evaluated for $Pe \gg 1$
%\Rightarrow \partd{j}\bar{u}_k=\frac{2\bar{u}_j}{R_j}\brc{ \delta_{jk} -2 \frac{R_k^2 L_j}{R_j^2 L_k} C_j \bra{ \vc{B}^T\brc{\vc{B} \vc{C} \vc{B}^T }^{\dagger}\vc{B}}_{jk}}\\
%\g{ 
%\partd{j}Pe_k=\frac{2Pe_j}{R_j}\brc{ \delta_{jk} -2\bra{ \frac{R_k}{R_j}}^2 C_i \bra{ \vc{B}^T\brc{\vc{B} \vc{C} \vc{B}^T }^{\dagger}\vc{B}}_{jk}}
%}

\end{document}
