# Supplementary material for: On biological flow networks: Antagonism between hydrodynamic and metabolic stimuli as driver of topological transitions
Source: arXiv:2111.04326 source file (2021-11-15)
Supplement: Supplementary file 3 [file S3-extraPlots.tex]

% % % % % % % % % % % % % % % % % % % % % % % %

\documentclass[10pt,letterpaper]{article}
\usepackage[left=0.9in, right=0.9in,]{geometry}
% amsmath and amssymb packages, useful for mathematical formulas and symbols
\usepackage{amsmath,amssymb}

% Use adjustwidth environment to exceed column width (see example table in text)
\usepackage{changepage}

% Use Unicode characters when possible
\usepackage[utf8x]{inputenc}

% textcomp package and marvosym package for additional characters
\usepackage{textcomp,marvosym}

% cite package, to clean up citations in the main text. Do not remove.
\usepackage{cite}

% Use nameref to cite supporting information files (see Supporting Information section for more info)
\usepackage{nameref,hyperref}

% line numbers
\usepackage[right]{lineno}

% ligatures disabled
\usepackage{microtype}
\DisableLigatures[f]{encoding = *, family = * }

% color can be used to apply background shading to table cells only
\usepackage[table]{xcolor}

% array package and thick rules for tables
\usepackage{array}

% create "+" rule type for thick vertical lines
\newcolumntype{+}{!{\vrule width 2pt}}

% create \thickcline for thick horizontal lines of variable length
\newlength\savedwidth

% \thickhline command for thick horizontal lines that span the table

% Remove comment for double spacing
%\usepackage{setspace} 
%\doublespacing

% Text layout
%\raggedright
%\setlength{\parindent}{0.5cm}
%\textwidth 5.25in 
%\textheight 8.75in

% Bold the 'Figure #' in the caption and separate it from the title/caption with a period
% Captions will be left justified
\usepackage[aboveskip=1pt,labelfont=bf,labelsep=period,justification=raggedright,singlelinecheck=off]{caption}

% Use the PLoS provided BiBTeX style
\bibliographystyle{plos2015}

% Remove brackets from numbering in List of References
\makeatletter
\renewcommand{\@biblabel}[1]{\quad#1.}
\makeatother

% Header and Footer with logo
\usepackage{lastpage,fancyhdr,graphicx}
\usepackage{epstopdf}
\pagestyle{fancy}
\fancyhf{}
%\setlength{\headheight}{27.023pt}
%\lhead{\includegraphics[width=2.0in]{PLOS-submission.eps}}
%\rfoot{\thepage/\pageref{LastPage}}
%\renewcommand{\headrulewidth}{0pt}
%\renewcommand{\footrule}{\hrule height 2pt \vspace{2mm}}
%\fancyheadoffset[L]{2.25in}
%\fancyfootoffset[L]{2.25in}
%\lfoot{\today}

%% END MACROS SECTION
\input{../packages}
\input{../macros}

\usepackage{comment}
\excludecomment{versiona}
\includecomment{versionb}

\begin{document}

\begin{LARGE}
\textbf{S3 Appendix: Concentrations, uptake and radial patterns in optimized flow networks}
\end{LARGE}

In the following section we present additional material on the systematic parameter scan of linkwise demand-supply adaptation, as described in the results section 2. 
The diagrams depict the nodal concentrations, uptake effectiveness and radial distributions for the selected $\sigma_0$, $\beta^*$, $\alpha_0$, $\alpha_1$ variations depicted in Fig. 3 and 4.
The $\chi$ notation depicts the relative distance of the respective vertex, or link center of the nearest source node, i.e. $\chi=0$ corresponds to a source node while $\chi=1$ describes sink-sided positions.

\begin{figure}[ht!]
\centering
\begin{versiona}
\subfloat[]{
\includegraphics[scale=1]{../Figures_Main/absorption_model/40875727/sweep_eval/profile_radii_grid}
 \label{fig:apx_screen12}}\\
\subfloat[]{
\includegraphics[scale=1]{../Figures_Main/absorption_model/40875727/sweep_eval/profile_uptake_grid}
 \label{fig:apx_screen13}}\\
\subfloat[]{
\includegraphics[scale=1]{../Figures_Main/absorption_model/40875727/sweep_eval/profile_concentration_grid}
 \label{fig:apx_screen14}}

\end{versiona}
\begin{versionb}
\subfloat{
 \label{fig:apx_screen12}}\\
\subfloat{
 \label{fig:apx_screen13}}\\
\subfloat{
 \label{fig:apx_screen14}}

\end{versionb}
\caption{
Radii, effective uptake and concentration profiles from source ($\chi=0$) to sink ($\chi=1$) for high demand and low absorption rates $\sigma_0=10^0$, $\beta^*=10^{-3}$, $\alpha_0= 4.5 \cdot 10^{-5}$, referring to the linkwise demand-supply scenario in hexagonal grids.}
\label{fig:apx_screen_networks_1}
\end{figure}

\begin{figure}[ht!]
\centering
\begin{versiona}
\subfloat[]{
\includegraphics[scale=1]{../Figures_Main/absorption_model/40881896/sweep_eval/profile_radii_grid}
 \label{fig:apx_screen22}}\\
\subfloat[]{
\includegraphics[scale=1]{../Figures_Main/absorption_model/40881896/sweep_eval/profile_uptake_grid}
 \label{fig:apx_screen23}}\\
\subfloat[]{
\includegraphics[scale=1]{../Figures_Main/absorption_model/40881896/sweep_eval/profile_concentration_grid}
 \label{fig:apx_screen24}}
\end{versiona}
\begin{versionb}
\subfloat{
 \label{fig:apx_screen22}}\\
\subfloat{
 \label{fig:apx_screen23}}\\
\subfloat{
 \label{fig:apx_screen24}}

\end{versionb}
 
\caption{
Radii, effective uptake and concentration profiles from source ($\chi=0$) to sink ($\chi=1$) for mediocre demand and mediocre absorption rates $\sigma_0=10^{-1}$, $\beta^*=10^{-2}$, $\alpha_0= 4.5 \cdot 10^{-5}$, referring to the linkwise demand-supply scenario in hexagonal grids.}
\label{fig:apx_screen_networks_2}
\end{figure}

\begin{figure}[ht!]
\centering
\begin{versiona}
\subfloat[]{
\includegraphics[scale=1]{../Figures_Main/absorption_model/40887599/sweep_eval/profile_radii_grid}
 \label{fig:apx_screen32}}\\
\subfloat[]{
\includegraphics[scale=1]{../Figures_Main/absorption_model/40887599/sweep_eval/profile_uptake_grid}
 \label{fig:apx_screen33}}\\
\subfloat[]{
\includegraphics[scale=1]{../Figures_Main/absorption_model/40887599/sweep_eval/profile_concentration_grid}
 \label{fig:apx_screen34}}
\end{versiona}
\begin{versionb}
\subfloat{
 \label{fig:apx_screen32}}\\
\subfloat{
 \label{fig:apx_screen33}}\\
\subfloat{
 \label{fig:apx_screen34}}
  
\end{versionb}
  \caption{Radii, effective uptake and concentration profiles from source ($\chi=0$) to sink ($\chi=1$) for low demand and high absorption rates $\sigma_0=10^{-2}$, $\beta^*=10^{-1}$, $\alpha_0= 8 \cdot 10^{-8}$, referring to the linkwise demand-supply scenario in hexagonal grids.}
\label{fig:apx_screen_networks_3}

\end{figure}

\end{document}
